# Supplementary material for: Resolving Ambiguity of the Kondo Temperature Determination in Mechanically Tunable Single-Molecule Kondo Systems
Source: arXiv:1811.00351 source file (2021-07-15)
Supplement: Supplementary file 1 [file SI.pdf]

# Following the Kondo temperature of a tunable single-molecule junction continuously from the Kondo singlet to the free spin 1/2 ground state - Supplementary Information

Martin Žonda,[1,*] Oleksandr Stetsovych,[2] Richard Korytár,[3] Markus Ternes,[4,5] Ruslan Temirov,[5,6] Andrea Racanelli,[5,6] Stefan Tautz,[5] Pavel Jelínek,[2,7] Tomáš Novotný,[3] and Martin Švec[2,7,†]

[1]*Institute of Physics, Albert Ludwig University of Freiburg, Hermann-Herder-Strasse 3, 79104 Freiburg, Germany*

[2]*Institute of Physics, Czech Academy of Sciences, Cukrovarnická 10, CZ-162 00 Praha 6, Czech Republic*

[3]*Department of Condensed Matter Physics, Faculty of Mathematics and Physics, Charles University, Ke Karlovu 5, CZ-121 16 Praha 2, Czech Republic*

[4]*Institute of Physics II B, RWTH Aachen University, 52074 Aachen, Germany*

[5]*Peter Grünberg Institut (PGI-3), Foschungszentrum Jülich, 52425 Jülich, Germany*

[6]*Jülich Aachen Research Alliance (JARA)–Fundamentals of Future Information Technology, 52425 Jülich, Germany*

[7]*RCPTM, Palacky University, Šlechtitelu 27, 783 71, Olomouc, Czech Republic.*

(Dated: November 1, 2018)

* martin.zonda@physik.uni-freiburg.de

† svec@fzu.cz

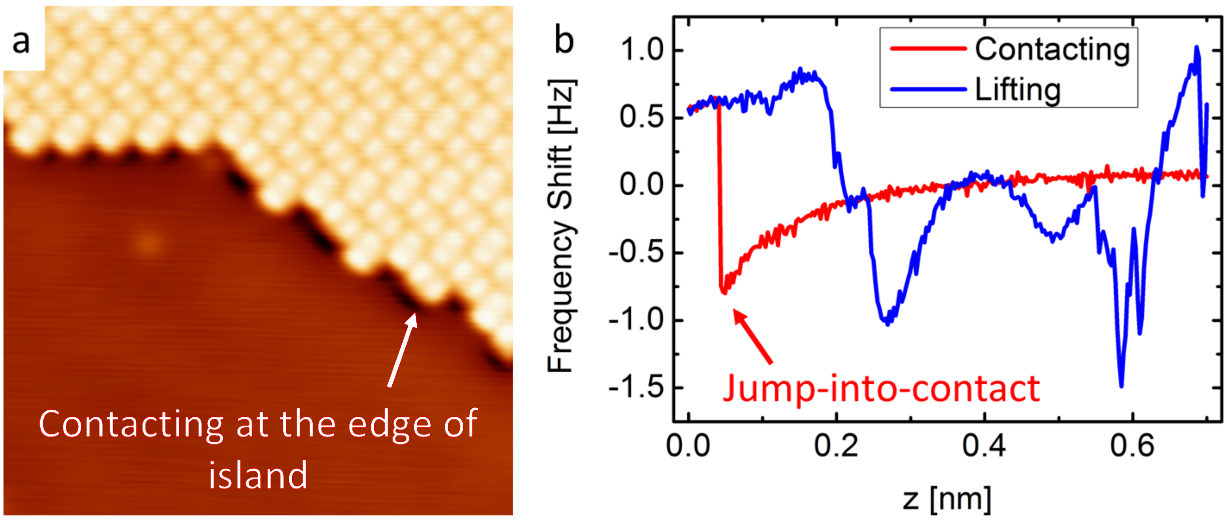


Supplementary Figure S1. The process of picking up a PTCDA molecule from the surface of Ag(111). a) STM topography image of a PTCDA island ($V = -350\,\mathrm{mV}$, $I = 50\,\mathrm{pA}$), with a molecule at the island boundary (marked by arrow), selected for the measurements. b) The frequency shift signal during the molecule lifting procedure, showing a jump-to contact event upon the tip approach (red) and the complex signal as a result of the PTCDA being lifted from the surface (blue).

## I. SAMPLE PREPARATION

PTCDA (4,9,10-perylenetetracarboxylic-dianhydride) molecules of 98% purity were evaporated in ultrahigh vacuum (UHV, $3 \times 10^{-10}\,\mathrm{mbar}$) from a Ta crucible at 670 K onto an atomically clean Ag(111) single-crystal surface kept at room temperature. Experiments were performed in UHV at a base temperature of 1.2 K using a combined atomic force and scanning tunneling microscope (AFM/STM) equipped with a $\mathrm{He}^4$-Joule-Thomson cooling stage (SPECS Surface Nano Analysis). The probing tip of the AFM/STM was treated before the experiment by repeatable interactions with clean Ag(111) surface until a stable metallic termination was reached. The contacting experiments were performed on PTCDA molecules on the edge of a molecular island, to minimize the chances of picking up the molecule after retraction of the tip (Fig. S1a). Each of the investigated PTCDA molecules was contacted by approaching the O site of the molecule with the probing tip until a jump-into-contact event was detected in the frequency shift channel (Fig. S1b). Once the contact was formed, $dI/dV(V, z)$ maps were recorded by changing consecutively sample bias $V$ and the lift distance $z$ without breaking the contact to the molecule. We note that $z = 400\,\mathrm{pm}$

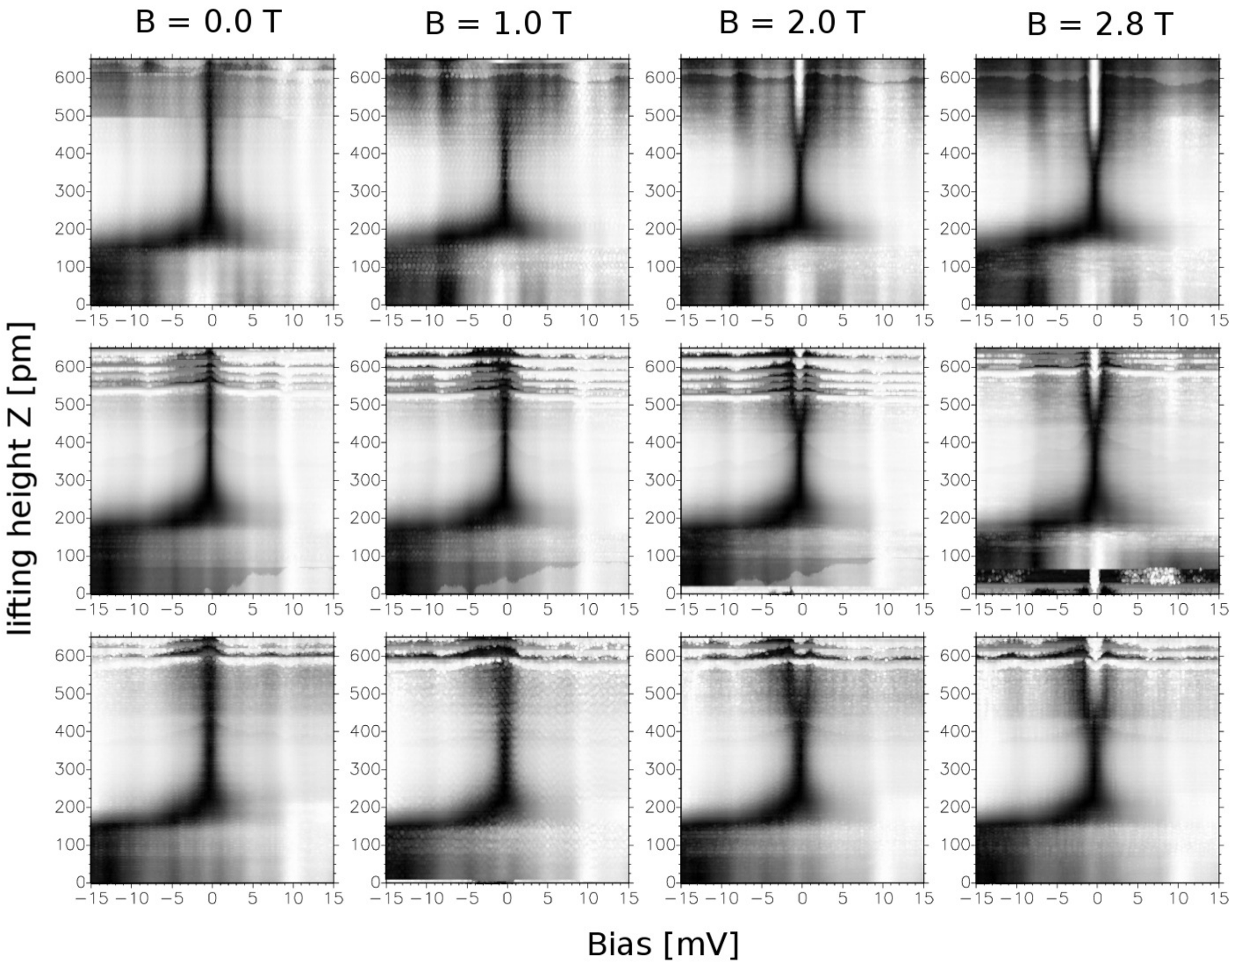


Supplementary Figure S2. Complete sets of the $dI/dV$ measurements taken with three different PTCDA molecules, at four levels of magnetic field. The intensities were normalized for each lifting distance separately. The digitization noise notable in the large lifting distance is an effect due to the normalization and the limited dynamic range of the used lock-in amplifier.

corresponds to the tip-sample distance over the PTCDA O-site at $I = 100\,\text{pA}$, $V = -350\,\text{mV}$ stabilization setpoint. The $dI/dV(V, z)$ maps were recorded on the same molecule at different magnetic fields ($B = 0, 1, 2, 2.8\,\text{T}$), see Fig. S2. During magnetic field changes the tip-PTCDA contact was loosed. Subsequently, we checked the surface area by rescanning before we recontacted the PTCDA molecule to insure that the molecule remained at the same position on the surface and that the tip structure did not change.

## II. MODEL AND FITTING PROCEDURE

We use a single-impurity Anderson model whose Hamiltonian reads

$$H = H_I + \sum_{\alpha=S,T} \left( H^b_\alpha + H^h_\alpha \right). \tag{S1}$$

Here, the first term describes the interacting lowest unoccupied molecular orbital (LUMO) of the PTCDA molecule,

$$H_I = \sum_\sigma \epsilon_d n_{d\sigma} + U n_{d\uparrow} n_{d\downarrow} + g\mu_B B S_z, \tag{S2}$$

where $d^\dagger_\sigma$ ($d_\sigma$) creates (annihilates) an electron with spin $\sigma$ in the LUMO at the energy $\epsilon_d$ and $n_{d\sigma} \equiv d^\dagger_\sigma d_\sigma$, $S_z \equiv (n_{d\uparrow} - n_{d\downarrow})/2$. $U$ represents the on-site repulsive Coulomb interaction between the electrons of opposite spin and the last term of Eq. (S2) accounts for the Zeeman energy due to an external magnetic field $B$.

The second term of Eq. (S1) describes the conduction bands of the substrate ($S$) and the tip ($T$) electrodes,

$$H^b_\alpha = \sum_{k,\sigma} \epsilon_{\alpha k} c^\dagger_{\alpha k\sigma} c_{\alpha k\sigma},$$

where $c^\dagger_{\alpha k\sigma}(c_{\alpha k\sigma})$ creates (annihilates) an electron with spin $\sigma$ in the state with momentum $k$ and the energy $\epsilon_{\alpha k\sigma}$. Finally, the last term in Eq. (S1) accounts for the hybridization between the conduction bands and the molecular orbital enabling electrical transport through the molecule

$$H^h_\alpha = \sum_{k,\sigma} \left( V_{\alpha k} d^\dagger_\sigma c_{\alpha k\sigma} + h.c. \right).$$

In our numerical calculations we assume energy-independent hybridization functions $\Gamma_\alpha(\epsilon) \equiv \pi \sum_k |V_{\alpha k}|^2 \delta(\epsilon - \epsilon_{\alpha k}) = \Gamma_\alpha$ and $\Gamma = \Gamma_S + \Gamma_T$ is the total hybridization.

The measured $dI/dV$ curves have been fitted using the formula for differential conductance in the tunneling regime [1, 2]

$$\frac{dI}{dV}(V) = G \int_{-\infty}^{\infty} d\omega\, \pi\Gamma\, \rho(\omega, \Gamma, T, B)(-f'(\omega - eV, T)), \tag{S3}$$

where the temperature- and magnetic-field-dependent spectral function $\rho_{\mathrm{NRG}}(\omega, \Gamma, T, B)$ calculated with numerical renormalization group theory (NRG) is convolved with the derivative of the Fermi-Dirac distribution to account for the broading during the tunneling process. We

used a band cut-off of $\pm 1\,\mathrm{eV}$ in the NRG calculations and assumed constant density of states. The NRG calculations have been performed using the open-source code NRG LJUBLJANA [3, 4]. The finite-temperature-dependent spectral functions have been calculated using the full density matrix algorithm based on the complete Fock-space concept [4, 5]. We have set the logarithmic discretization parameter $\Lambda = 2$ and used the interleaved method [6, 7] to smoothen the spectral functions calculated for a dense mesh of $\Gamma$ values.

Here we shortly discuss the approximations introduced to make the comparison between the experiment and model possible:

(i) We consider only a constant hybridization function. It has been shown in a recent study of a similar system (Au-PTCDA complex) [2] that the replacement of the function $\Gamma(\omega)$ by its value at the Fermi energy may lead to a factor 1.5 difference in $T_{\mathrm{K}}$. However, considering that in our study $T_{\mathrm{K}}$ changes by more than nine orders of magnitude, such a correction would not alter our conclusions.

(ii) We have truncated the parametric space by fixing the values of all parameters except $\Gamma$ and $G$. As revealed by an ab-initio study of the tip/PTCDA/Ag junction [8] the $U$ can vary with increasing $z$. We have made a complete analysis for $U = 0.5\,\mathrm{eV}$ and $U = 1\,\mathrm{eV}$, which represent a relevant range of values extrapolated from the cited study. Because $U$ does not significantly affect the results (see Fig. S3a), we present in the main text only the results for $U = 1\,\mathrm{eV}$.

(iii) Because the experimentally measured Kondo resonances are nearly symmetric with respect to the Fermi level, we have assumed electron-hole symmetry and fixed the "half-filling" condition $\epsilon_d = -U/2$. This allows us to approximate the Kondo temperature by [9, 10]

$$T_{\mathrm{K}} = 0.29\sqrt{\Gamma U}\exp\left(-\frac{\pi U}{8\Gamma}\right). \tag{S4}$$

A small systematical offset of the peak position with respect to zero bias has been accounted for by shifting the data by a constant energy of $-0.26\,\mathrm{meV}$.

(iv) We have used the gyromagnetic factor $g = 2$ for the free electronic spin. We have tested this value using a perturbative fitting procedure introduced by one of the coauthors [11]. Note that the true $g$-factor can slightly differ from this value because of the exchange interaction with the conduction electrons polarized by the magnetic field [12].

(v) Finally, we note that the best temperature to describe the spectra of the PTCDA molecule either with Eq. (S3) or with the perturbative scattering model of Ref. [11] is

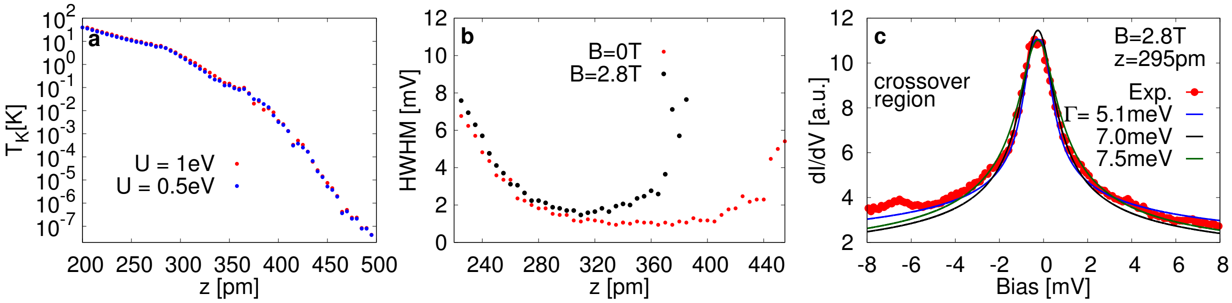


Supplementary Figure S3. a) Comparison of $T_K$ fitted with $U = 0.5\,\mathrm{eV}$ and $U = 1\,\mathrm{eV}$. b) HWHM obtained directly from the experimental data for $B = 0$ and $2.8\,\mathrm{T}$. The magnetic field leads to a splitting of the conductance peak at $z \approx 400\,\mathrm{pm}$. Therefore, the HWHM is not well defined for $B = 2.8\,\mathrm{T}$ at $z \gtrsim 400\,\mathrm{pm}$. c) The experimental $dI/dV$ from the crossover region fitted with different $\Gamma$'s. The example $z = 295\,\mathrm{pm}$ is close to the apparent step in the inset of Fig. 4a in the main text.

$T_{\mathrm{exp}} = 1.4\,\mathrm{K}$ slightly above the base temperature of $1.2\,\mathrm{K}$ of the experimental setup.

## III. FITTING IN THE CROSSOVER REGION

The width of the zero-bias conductance peak is in the crossover regime, where $T_{\mathrm{K}} \sim T_{\mathrm{exp}}$, not very sensitive to $T_{\mathrm{K}}$. Therefore, we have found that the half-width at half-maximum (HWHM) obtained from the experimental data shows a broad, plateau-like minimum and even increases for sufficiently large $z$ (Fig. S3b). This non-monotonous behavior is an indirect consequence of the decreasing ratio of $T_{\mathrm{K}}/T_{\mathrm{exp}}$ which leads to decreasing intensity of the zero bias Kondo peak. Whereas for $T_{\mathrm{K}} \gg T_{\mathrm{exp}}$ the HWHM is directly proportional to $T_{\mathrm{K}}$, the width of the observed Kondo peak at $T_{\mathrm{K}} \lesssim T_{\mathrm{exp}}$ is primarily defined by $T_{\mathrm{exp}}$. Even worse, because the Kondo peak intensity rapidly decreases with further reduction of $T_{\mathrm{K}}$ and the shape of the peak develops to a temperature broadened logarithm [11, 13], the HWHM measured at a fixed energy range around zero apparently *increases*. This counterintuitive behavior is displayed in Fig. S3b and is also visible in the Frota fits shown in Fig. 2a of the main text.

To overcome this problem of determining $T_K$, we apply an external magnetic field $B$ strong enough to split the Kondo peak in the weak-coupling regime, that means the Zeeman energy has to be sufficiently larger than the thermal energy, $g\mu_{\mathrm{B}}B \gtrsim 2k_{\mathrm{B}}T_{\mathrm{exp}}$. In such a

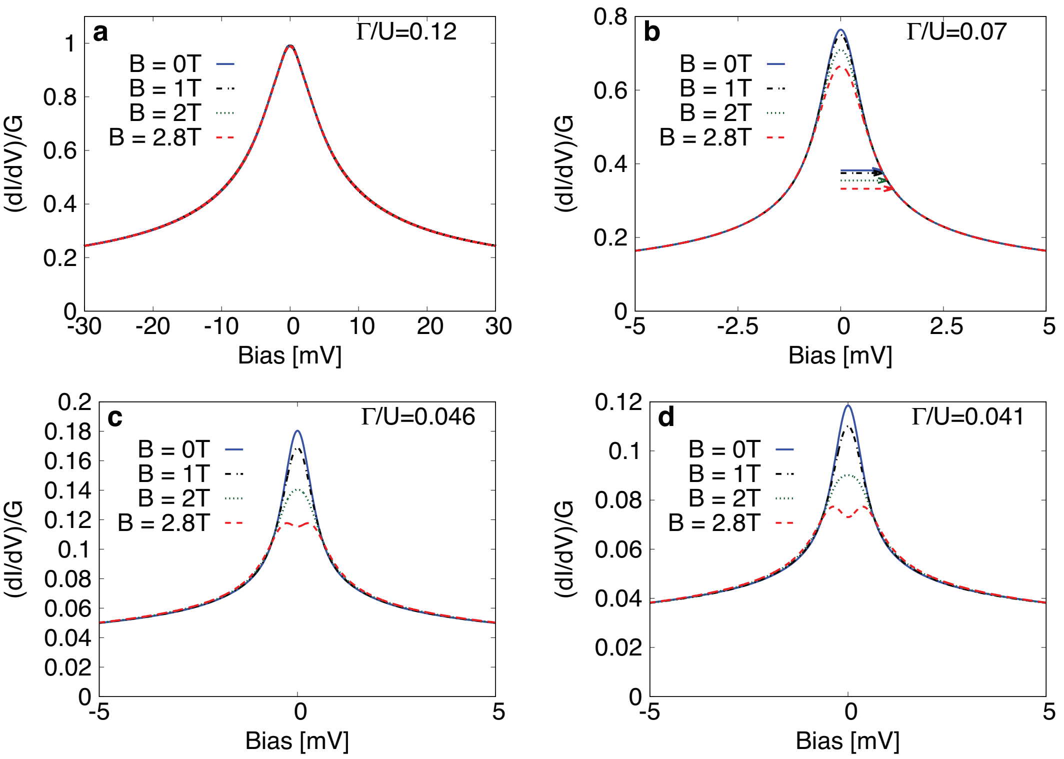


Supplementary Figure S4. NRG-based $dI/dV$ simulations at different $\Gamma/U$ ratios and magnetic fields $B$. a) At $\Gamma/U = 0.12$ the system remains even at $B = 2.8$ T in the strong coupling regime with $k_\mathrm{B}T_\mathrm{K} \gg g\mu_\mathrm{B}B$ and the spectra at different $B$ are indistinguishable. b) In the crossover regime ($\Gamma/U = 0.07$) with $2k_\mathrm{B}T_\mathrm{K} \approx g\mu_\mathrm{B}B$ only the central peak intensity is reduced. Note, that the HWHM, signalled by arrows, effectively increases with B. c)+d) In the weak coupling limit ($\Gamma/U \leq 0.046$) with $k_\mathrm{B}T_\mathrm{K} \ll g\mu_\mathrm{B}B$ the split can be observed as soon as $2k_\mathrm{B}T_\mathrm{exp} \lesssim g\mu_\mathrm{B}B$.

$B$-field we can distinguish two clear limits (see Fig. S4):

(i) A Kondo system in which the peak show no splitting *and* in which the HWHM is sufficiently larger than $k_\mathrm{B}T_\mathrm{exp}$ can be safely assumed to be in the strong-coupling regime where $T_K$ is determined by the HWHM of the peak (Fig. S4a).

(ii) An observed split peak indicates a Kondo effect in the weak-coupling regime with $2k_BT_K \lesssim g\mu_\mathrm{B}B$. In this regime the HWHM is not a good indicator for $T_K$. However, using NRG-based or perturbative models the true $T_K$ can be determined (Fig. S4c-d).

However, in the crossover regime, where the HWHM is not a good quantity for $T_\mathrm{K}$ because $T_\mathrm{K} \sim T_\mathrm{exp}$, often also the experimentally available external field is only $k_\mathrm{B}T_\mathrm{K} \sim g\mu_\mathrm{B}B$, and therefore not strong enough to visibly split the peak. In this situation, neither of

the two cases above is applicable. This is demonstrated in Fig. S3c where we plot data measured at $z = 295\,\mathrm{pm}$ and at $B = 2.8\,\mathrm{T}$. The Kondo peak is not split, however, the HWHM is with $\approx 1.6\,\mathrm{mV}$ only a factor 4 above the minimal experimental broadening of $3.5 k_\mathrm{B} T_\mathrm{exp}/e = 0.42\,\mathrm{mV}$. Therefore, we can fit the data with a large variance in $\Gamma$ — all three displayed curves fit the experimental data equally well, even thought their coupling to the substrate ranges from $\Gamma = 5.1\,\mathrm{meV}$ to $7.5\,\mathrm{meV}$ leading via Eq. (S4) to an order of magnitude difference in $T_\mathrm{K}$ and to the apparent step in the "direct-fit" curve shown in the inset of Fig. 4a of the main text.

Although the HWHM is not very sensitive to the change of $T_\mathrm{K}$ in the crossover region, the amplitude of the peak depends strongly on the external field $B$ (see Fig. S4b and c and Fig. 4c of the main text). This enables us to compare the ratio of $dI/dV(V = 0\,\mathrm{mV})$ measured in two sufficiently different magnetic fields with theory calculations to determine the correct $\Gamma$. We note that it is crucial to use the ratio of two experimental sets to be independent of the total amplitude parameter $G$ in Eq. (S3). The black curve in Fig. S3c shows the best fit using the above method.

## IV. VOLTAGE – ASYMMETRIC VIBRATIONAL SIGNAL

The experimental $dI/dV$ (Figs. 2 and 3 in the main text) reveal, additionally to the central resonance, peaks and dips at finite bias which we attribute to excitations of vibrational modes in the molecular junction. We observe peaks at roughly $-7\,\mathrm{meV}$ and shallow dips around $+7\,\mathrm{meV}$ which do not change with increasing magnetic field and only weakly respond to stretching, mainly by a non-monotonous shift of the excitation energy, similar to Ref. [14].

The asymmetry of the vibrational pairs in the inelastic electron tunneling spectroscopy (IETS) was considered theoretically by Paulsson *et al.* within the self-consistent Born approximation and the lowest-order expansion [15]. Their methodology has been applied in the analysis of asymmetries in the IETS by Xu *et al.* [16]. To proceed with the analysis of Paulsson *et al.* [15], we employ a simple model of the molecule which contains a single (frontier) orbital that is coupled to a single vibrational mode and a pair of leads. The resulting $\mathrm{d}I/\mathrm{d}V$ can be decomposed as

$$\begin{aligned} \frac{\mathrm{d}I}{\mathrm{d}V}(V) = {} & \frac{2e^2}{h}\tau \\ & + W^{(S)} G^{(S)}(eV, \hbar\omega, k_B T) + W^{(A)} G^{(A)}(eV, \hbar\omega, k_B T), \end{aligned} \tag{S5}$$

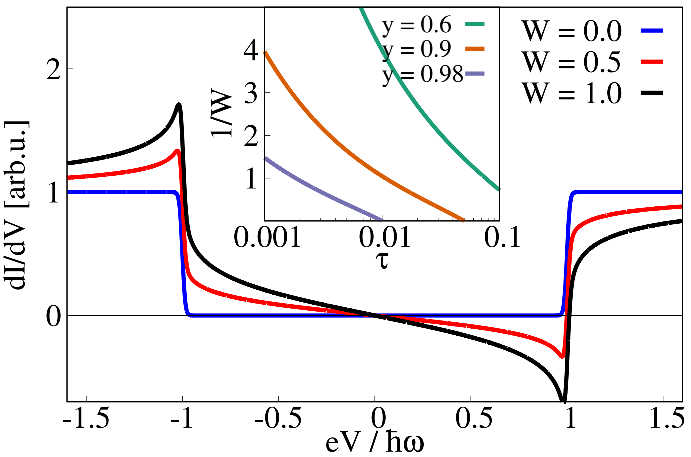


Supplementary Figure S5. Inelastic contribution to the differential conductance calculated from Ref. [15] for different relative weights of the anti-symmetric part $W \equiv W^{(A)}/W^{(S)}$. The unit of energy $\hbar\omega$ is the energy of the vibrational excitation. The broadening is solely due to the temperature, which we set to $k_{\mathrm{B}}T = \hbar\omega/50$. *Inset:* Dependence of $1/W$ on electronic parameters: the elastic Landauer transmission $\tau$ and the coupling imbalance $y \equiv |\Gamma_T - \Gamma_S|/(\Gamma_T + \Gamma_S)$.

where the first part is the elastic Landauer term ($\tau$ being the transmission) and the remaining two terms are due to inelastic processes involving the vibration. The functions $G^{(S/A)}$ are symmetric and anti-symmetric in voltage and are universal in the sense that they do not depend on microscopic parameters other than the vibrational frequency $\omega$ and the temperature $T$. The symmetric and anti-symmetric lineshapes combine with weights $W^{(S/A)}$. We plot the inelastic part in Fig. S5 for different ratios $W^{(A)}/W^{(S)} = W$. The ratio $W$ depends only on electronic parameters, namely, the (orbital) line-widths $\Gamma_T$ and $\Gamma_S$ due to the tip and the substrate, respectively, and the orbital (on-site) energy $\epsilon_d$. In the inset of Fig. S5 we plot $1/W$ expressed as a function of the coupling imbalance $y \equiv |\Gamma_T - \Gamma_S|/(\Gamma_T + \Gamma_S)$ and the elastic Landauer transmission $\tau$. The model predicts that the anti-symmetric signal gets more prominent (large $W$) when the coupling imbalance $y$ is large and $\tau$ is low.

This prediction can be compared with the experimental $dI/dV$ (Fig. 2, main text). The asymmetry of the inelastic signal is clearly visible when $z \lesssim 350\,\mathrm{nm}$. The elastic transmission can be estimated from the $dI/dV$ in units of $G_0$ at $\pm 15\,\mathrm{mV}$, where we get $\tau \gtrsim 10^{-2}$. Additionally, the imbalance $y$ can be readily obtained from the fitted values of $\Gamma_T$ and $\Gamma_S$ displayed in Fig. 5 of the main text. For $z \lesssim 350\,\mathrm{nm}$ $y$ approaches 0.9. According to the

inset of Fig. S5, these estimates of $\tau$ and $y$ imply that $W^{(A)} \approx W^{(S)}$, which is in agreement with the observed asymmetry of the inelastic signal.

However, we emphasize that the comparison can only be made on a qualitative level, because the model by Paulsson *et al.* [15] does not apply to the Coulomb blockade, i. e. to an open shell molecule. The treatment of vibrational coupling in the Coulomb blockade with a fully developed Kondo resonance presents an open theoretical problem.

---


[1] A. Schiller and S. Hershfield, Phys. Rev. B **61**, 9036 (2000).

[2] T. Esat, T. Deilmann, B. Lechtenberg, C. Wagner, P. Krüger, R. Temirov, F. B. Anders, M. Rohlfing, and F. S. Tautz, Phys. Rev. B **91**, 144415 (2015).

[3] R. Žitko and T. Pruschke, Phys. Rev. B **79**, 085106 (2009).

[4] R. Žitko, "NRG Ljubljana - open source numerical renormalization group code," (2014), http://nrgljubljana.ijs.si.

[5] A. Weichselbaum and J. von Delft, Phys. Rev. Lett. **99**, 076402 (2007).

[6] V. L. Campo and L. N. Oliveira, Phys. Rev. B **72**, 104432 (2005).

[7] R. Žitko, Comp. Phys. Comm. **180**, 1271 (2009).

[8] A. Greuling, M. Rohlfing, R. Temirov, F. S. Tautz, and F. B. Anders, Phys. Rev. B **84**, 125413 (2011).

[9] F. D. M. Haldane, Journal of Physics C: Solid State Physics **11**, 5015 (1978).

[10] H. R. Krishna-murthy, J. W. Wilkins, and K. G. Wilson, Phys. Rev. B **21**, 1003 (1980).

[11] M. Ternes, New J. Phys. **17**, 063016 (2015).

[12] E. L. Wolf and D. L. Losee, Phys. Lett. A **29**, 334 (1969).

[13] Y. Zhang, S. Kahle, T. Herden, C. Stroh, M. Mayor, U. Schlickum, M. Ternes, P. Wahl, and K. Kern, Nature Comm. **4**, 2110 (2013).

[14] D. Rakhmilevitch, R. Korytár, A. Bagrets, F. Evers, and O. Tal, Phys. Rev. Lett. **113**, 236603 (2014).

[15] M. Paulsson, T. Frederiksen, and M. Brandbyge, Phys. Rev. B **72**, 201101 (2005); in *Journal of Physics: Conference Series*, Vol. 35 (IOP Publishing, 2006) p. 247.

[16] C. Xu, C.-l. Chiang, Z. Han, and W. Ho, Phys. Rev. Lett. **116**, 166101 (2016).
